# Supplementary material for: Matrix product states with large sites
Source: arXiv:2109.11036 ancillary file (2022-01-21)
Supplement: Supplementary file 1 [file ESI.pdf]

# Supporting Information for:
# Matrix product states with large sites

Henrik R. Larsson,[1,a)] Huanchen Zhai,[1] Klaas Gunst,[1,2,3,b)] and Garnet Kin-Lic Chan[1,c)]

[1)] *Division of Chemistry and Chemical Engineering, California Institute of Technology, Pasadena, CA 91125, USA*

[2)] *Center for Molecular Modeling, Ghent University, Technologiepark 46, B-9052 Zwijnaarde, Belgium*

[3)] *Department of Physics and Astronomy, Ghent University, Krijgslaan 281, S9, B-9000 Ghent, Belgium*

(Dated: 22 September 2021)

## ADDITIONAL DATA FOR THE CHROMIUM DIMER

TABLE I. Energies in $E_H$ for the chromium dimer at the MPS-MRCISD+$Q_P$ level of theory for various cc-p$n$Z-DK bases. "5Z(extrap)" denotes the energy for the cc-pV5Z-DK basis after extrapolating the bond dimension to $\infty$.

| $R$/Å | DZ | TZ | QZ | 5Z | 5Z(extrap) | error 5Z extrap |
|---|---|---|---|---|---|---|
| 1.5 | -2099.8945 | -2100.1811 | -2100.3137 | -2100.3861 | -2100.3932 | 0.0016 |
| 1.6 | -2099.9174 | -2100.2023 | -2100.3328 | -2100.4045 | -2100.4123 | 0.0018 |
| 1.7 | -2099.9215 | -2100.2051 | -2100.3334 | -2100.4046 | -2100.4119 | 0.0017 |
| 1.8 | -2099.9186 | -2100.2013 | -2100.3277 | -2100.3981 | -2100.4055 | 0.0017 |
| 2.0 | -2099.9105 | -2100.1929 | -2100.3165 | -2100.3856 | -2100.3919 | 0.0015 |
| 2.1 | -2099.9075 | -2100.1906 | -2100.3133 | -2100.3822 | -2100.3873 | 0.0012 |
| 2.2 | -2099.9054 | -2100.1897 | -2100.3116 | -2100.3794 | -2100.3839 | 0.0011 |
| 2.4 | -2099.9024 | -2100.1895 | -2100.3105 | -2100.3786 | -2100.3818 | 0.0009 |
| 2.5 | -2099.9010 | -2100.1894 | -2100.3102 | -2100.3787 | -2100.3819 | 0.0008 |
| 2.7 | -2099.8980 | -2100.1882 | -2100.3085 | -2100.3769 | -2100.3809 | 0.0010 |
| 2.9 | -2099.8936 | -2100.1854 | -2100.3058 | -2100.3738 | -2100.3747 | 0.0004 |
| 3.1 | -2099.8886 | -2100.1818 | -2100.3022 | -2100.3695 | -2100.3706 | 0.0004 |
| 3.5 | -2099.8793 | -2100.1745 | -2100.2949 | -2100.3629 | -2100.3629 | 0.0001 |
| $\infty$ | -2099.8648 | -2100.1626 | -2100.2800 | -2100.3503 | | |
| atom | -1049.9316 | -1050.0835 | -1050.1442 | -1050.1785 | | |

[a)] Electronic mail: larsson [a t] caltech . eδu
[b)] Present address: Quantum Simulation Technologies, Inc., Cambridge, MA 02139; Present address: Quantum Simulation Technologies, Inc., Cambridge, MA 02139
[c)] Electronic mail: garnetc [a t] caltech . eδu

TABLE II. Energies in $E_H$ for the chromium dimer using the cc-pVDZ-DK basis.

| $R$/Å | MPS-MRCISD | $+Q_D$ | $+Q_{RD}$ | $+Q_M$ | $+Q_P$ | MPS-MRCISDT |
|---|---|---|---|---|---|---|
| 1.5 | -2099.8150 | -2099.8824 | -2099.8911 | -2099.8805 | -2099.8945 | -2099.9311 |
| 1.6 | -2099.8366 | -2099.9048 | -2099.9139 | -2099.9030 | -2099.9174 | -2099.9536 |
| 1.7 | -2099.8400 | -2099.9086 | -2099.9178 | -2099.9069 | -2099.9215 | -2099.9568 |
| 1.8 | -2099.8372 | -2099.9056 | -2099.9148 | -2099.9040 | -2099.9186 | -2099.9529 |
| 2.0 | -2099.8317 | -2099.8979 | -2099.9068 | -2099.8963 | -2099.9105 | -2099.9426 |
| 2.1 | -2099.8310 | -2099.8955 | -2099.9041 | -2099.8939 | -2099.9075 | -2099.9385 |
| 2.2 | -2099.8312 | -2099.8940 | -2099.9022 | -2099.8923 | -2099.9054 | -2099.9352 |
| 2.4 | -2099.8326 | -2099.8922 | -2099.8997 | -2099.8903 | -2099.9024 | -2099.9294 |
| 2.5 | -2099.8328 | -2099.8912 | -2099.8985 | -2099.8892 | -2099.9010 | -2099.9272 |
| 2.7 | -2099.8319 | -2099.8886 | -2099.8956 | -2099.8867 | -2099.8980 | -2099.9217 |
| 2.9 | -2099.8295 | -2099.8848 | -2099.8914 | -2099.8828 | -2099.8936 | -2099.9157 |
| 3.1 | -2099.8263 | -2099.8802 | -2099.8866 | -2099.8781 | -2099.8886 | -2099.9094 |
| 3.5 | -2099.8199 | -2099.8717 | -2099.8776 | -2099.8695 | -2099.8793 | -2099.8985 |
| $\infty$ | -2099.8093 | -2099.8582 | -2099.8636 | -2099.8559 | -2099.8648 | -2099.8899 |
| atom | -1049.9167 | -1049.9323 | -1049.9333 | -1049.9287 | -1049.9316 | -1049.9416 |
